# Supplementary material for: Physical Adversarial Camouflage through Gradient Calibration and Regularization
Source: arXiv:2508.05414 source file (2025-08-07)
Supplement: Supplementary file 1 [file 07-Appendix.tex]

\section{Appendix}\label{sec: appendix}
